# Supplementary material for: Will This Video Go Viral? Explaining and Predicting the Popularity of Youtube Videos
Source: arXiv:1801.04117 source file (2018-03-01)
Supplement: Supplementary file 1 [file appendix.tex]

%!TEX root = sir-hawkes.tex
%
\newpage
\appendix
\etocdepthtag.toc{mtappendix}
\etocsettagdepth{mtchapter}{none}
\etocsettagdepth{mtappendix}{subsection}
\etoctocstyle{1}{Contents (Appendix)}
\tableofcontents‎‎

\section{Inter-event time probabilities in non-homogeneous Poisson processes}
\label{ap-subsec:probs-NHPP}

In this section, we revisit the Non-Homogeneous Poisson Process (NHPP) and we compute the formula for the probabilities of observing inter-arrival times.
We also show that NHPP is a non-Markovian process and we derive a simple proof for the formula for the log-likelihood of a NHPP, which is widely used in CS literature, but an accessible proof of which is currently missing.

\subsection{Inter-arrival times probabilities}

Here we compute the probability of observing $t_i$ -- the arrival of an event.
We denote by $\tau_i$ the inter-arrival time between event $i-1$ and event $i$.
It follows that $\tau_i = t_i - t_{i-1}$ and $t_i = \sum_1^j \tau_j$.
We study in parallel the Homogeneous Poisson Process (HPP) and NHPP.
For ease of understanding, we further consider the two cases when $i = 1$ and $i > 1$.

\textbf{The arrival of the first event $t_1$}.
In a HPP of intensity $\lambda$, the probability of having no events in the time interval $[0, t)$ is:
\begin{equation} \label{eq:CCDF-waiting-time}
	\mathbbm{P}[t_1 \ge t] = e^{-\lambda t} \enspace .
\end{equation}
This can be interpreted as the probability of waiting at least $t$ units of time until the first event.
Consequently, Eq.~\eqref{eq:CCDF-waiting-time} is the CCDF (Complementary Cumulative Distribution Function) of the waiting time until the first event.
The PDF is $ PDF = \fp{}{t} (1 - CCDF) = - \fp{}{t} CCDF$.
Consequently \emph{the waiting time to the first event in a HPP is distributed exponentially}, with parameter $\lambda$:
\begin{equation}
	\mathbbm{P}[t_1 = t] = - e^{-\lambda t} \fp{-\lambda t}{t} = \lambda e^{-\lambda t} \enspace.
\end{equation}

For a NHPP with the event rate $\lambda(t)$, we first define the function $\Lambda(t) = \int_0^t \lambda(\tau) d\tau$.
The inverse relation between $\lambda(t)$ and $\Lambda(t)$ is $\lambda(t) = \fp{}{t} \Lambda(t)$.
We have:
\begin{equation} \label{eq:NHPP-wait-0-t}
	\mathbbm{P}[t_1 \ge t] = e^{-\Lambda(t)} \enspace ,
\end{equation}
and we compute
\begin{equation} \label{eq:NHPP-waiting-t1}
	\mathbbm{P}[t_1 = t] = \fp{}{t} e^{-\Lambda(t)} = - e^{-\Lambda(t)} \fp{}{t} \Lambda(t) = \lambda(t) e^{-\Lambda(t)} \enspace.
\end{equation}
Note that \emph{the waiting time to the first event is not exponentially distributed in the case of NHPP}.
An intuitive interpretation of Eq.~\eqref{eq:NHPP-waiting-t1} is that the probability of observing an event at time $t$ is the product of 
the probability of observing an event in the infinitesimal time interval  $[t, t + \partial t]$ -- equal to the event rate $\lambda(t)$ --
and the probability having observed no event in $[0, t]$ -- as defined in Eq.\eqref{eq:NHPP-wait-0-t}.
%
%\begin{figure}[tbp]
%	\centering
%	\includegraphics[width=0.3\textwidth]{Lambda-of-t}
%	
%	\caption{
%		Graphical representation of the relation between the functions $\lambda(t)$ (the intensity function of a NHPP) and $\Lambda(t)$ used in Sec.~\ref{ap-subsec:probs-NHPP} to compute the inter-arrival time probabilities in a NHPP.
%	}
%	\label{fig:Lambda}
%\end{figure}

\textbf{The arrival of $t_2, t_3, \ldots, t_n$}.
For a HPP of rate $\lambda$, the probability of not observing an event in the interval $[t, t + s]$ -- after having observed a first event at time $t_1 = t$ -- is:
\begin{equation*}
	\mathbbm{P}[t_2 - t_1 \ge s | t_1 = t] = e^{- \lambda (t+s - t)} = e^{- \lambda s} \enspace .
\end{equation*}
does not depend of $t$. By denoting $\tau_2 = t_2 - t_1$ and $\tau_1 = t_1$, we obtain
\begin{equation} \label{eq:HPP-inter-arrival-times-prob-distribution}
	\mathbbm{P}[\tau_2 = s | \tau_1 = t] = \lambda e^{- \lambda s} \Longrightarrow \mathbbm{P}[\tau_i = s ] = \lambda e^{- \lambda s} \enspace.
\end{equation}
Inter-arrival times in a HPP are exponentially distributed with parameters $\lambda$, and the probability of observing a $\tau_i$ does not depend on the previous inter-arrival times $\tau_1, \tau_2, \ldots, \tau _{i-1}$.
This property is called \emph{memorylessness} -- and it is equivalent to the Markovian property~\cite{Allen2008} -- as the next state of the process depends only on the current state and not on the past.

For the NHPP of rate $\lambda(t)$, we have
\begin{align}
	\mathbbm{P}[t_2 - t_1 \ge s | t_1 = t] &= e^{ \Lambda (t) - \Lambda(t+s)} \nonumber \\
	\Rightarrow \;  \mathbbm{P}[t_2 - t_1 = s | t_1 = t] &= \fp{}{s} \mathbbm{P}[t_2 - t_1 \ge s | t_1 = t] \nonumber \\
	 &= \lambda(t+s) e^{ \Lambda (t) - \Lambda(t+s)} \nonumber
\end{align}
$\Lambda (t) - \Lambda(t+s)$ can be interpreted as the minus area under the curve of $\lambda(t)$. %, as can be seen in Fig.~\ref{fig:Lambda}.
We can further show that
\begin{equation} \label{eq:NHPP-inter-event-times-prob}
	\mathbbm{P}[\tau_{i+1} = s | \mathcal{H}_i] = \lambda(t_i+s) e^{ \Lambda (t_i) - \Lambda(t_i+s)} 
\end{equation}
where $\mathcal{H}_i = \{ t_1, t_2, \ldots, t_i\}$ is the history of the process up to event $t_i$. 
Note that when $\lambda(t) = \lambda$ -- i.e. a HPP -- we have $\Lambda(t) = \lambda t$ and Eq.~\ref{eq:HPP-inter-arrival-times-prob-distribution} and~\ref{eq:NHPP-inter-event-times-prob} are identical.
We can express Eq.~\eqref{eq:NHPP-inter-event-times-prob} in terms of event times (rather than inter-event times):
\begin{equation} \label{eq:NHPP-event-times-prob}
	\mathbbm{P}[t_{i+1} | \mathcal{H}_i] = \lambda(t_{i+1}) e^{ \Lambda (t_i) - \Lambda(t_{i+1})} 
\end{equation}

\subsection{Two follow-up conclusions}

We study the Markovian property of NHPP and we derive its likelihood function.

\textbf{NHPP is not Markovian}.
One direct consequence of Eq~\eqref{eq:NHPP-inter-event-times-prob} is that inter-arrival times in a NHPP are not exponentially distributed.
We further study if the process is memoryless -- i.e. if it has the Markovian property.
For this, we compute the join probability of having an event in the interval $[0, t]$ and a second event in $[t, s]$.
\begin{align}
	\mathbbm{P}[t_1 = t, t_2 = t + s] &= \mathbbm{P}[t_1 = t] \mathbbm{P}[t_2 = t + s | t_1 = t] \nonumber \\ 
	&= \lambda(t) \lambda(t + s) e^{- \Lambda(t + s)} \label{eq:non-markov}
\end{align}
which shows that $t_2$ is not independent of $t_1$.
The implication is that the next state of a NHPP -- i.e. $t_{i+1}$ -- is dependent on all previous states -- $t_j, j \in [1 \dots i]$.
\emph{This shows that NHPP is not Markovian.}
Note that this is a general results, for non-specific functions $\lambda(t)$
Specific functions $\lambda(t)$ can be constructed so that the NHPP becomes Markovian.

As a sanity check, we write Eq.~\eqref{eq:non-markov} for a HPP.
We obtain
\begin{align}
	\mathbbm{P}[t_1 = t, t_2 = t + s] &= \lambda ^2 e^{-\lambda (t+s)} \nonumber \\
	&= \lambda e^{-\lambda t} \lambda e^{- \lambda s} = \mathbbm{P}[t_1 = t] \mathbbm{P}[t_2 = t + s]
\end{align}
therefore the inter-arrival times $\tau_1$ and $\tau_2$ are independent and exponentially distributed -- as expected.

\textbf{The likelihood function for NHPP}.
Given $\mathcal{H}_i$, which includes the parameter of the process $\theta$ and the history of the process up to event $t_i$, the probability of an event at time $t_{i+1}$ is defined (according to Eq.~\eqref{eq:NHPP-event-times-prob} as the probability of observing an event at time $t_{i+1}$ -- $\Lambda(t_{i+1})$ -- and the probability of not having observed any event in the interval $[t_i, t_{i+1}]$.

We construct the likelihood function as
\begin{align}
	Likelihood(\theta) &= \mathbbm{P}[t_1, t_2, \dots, t_n | \theta] \nonumber \\
	&= \mathbbm{P}[t_1 | \theta] \mathbbm{P}[t_2 | t_1, \theta] \mathbbm{P}[t_3 | t_2, t_1, \theta] \ldots \mathbbm{P}[t_n | t_{n-1}, \ldots t_1, \theta] \nonumber \\
	&= \prod_{i = 1}^n \mathbbm{P}[t_i | \mathcal{H}_{i-1}] = e^{-\Lambda(t_1)+\Lambda(t_1)-\Lambda(t_2) + \ldots - \Lambda(t_n)} \prod_{i = 1}^n \lambda(t_i) \nonumber \\
	&= \prod_{i = 1}^n \lambda(t_i) e^{-\Lambda(t_n)} \nonumber
\end{align}
Finally, we derive the expression of the log-likelihood widely used in literature:
\begin{align} 
	log(Likelihood(\theta)) &= \sum_{i = 1}^n log \left( \lambda(t_i) \right) - \Lambda(t_n) \nonumber \\
	&= \sum_{i = 1}^n log \left( \lambda(t_i) \right) - \int_0^{t_n} \lambda(\tau)d\tau . \label{eq:log-likelihood}
\end{align}

\section{Fitting HawkesN with AMPL -- implementation}
We fit the parameters of the HawkesN model to observed data by maximizing the log-likelihood function Eq.~\eqref{eq:log-likelihood}. 
We use AMPL, an industry standard for modeling optimization problems and with a transparent interfaces to powerful solvers.
We start with an introduction of AMPL (Sec.~\ref{subsec:ampl-intro}), we describe our optimization setup and the employed solvers (Sec.~\ref{subsec:optimization-setup}) and we finish with the R interface that we constructed for AMPL (Sec.~\ref{subsec:ampl-r-interface}).

\subsection{AMPL introduction}
\label{subsec:ampl-intro}
Since the first commercial release in 1993, AMPL -- which stands for A Mathematical Programming Language -- has provided a convenient interface between mathematic modelers and implemented solvers~\cite{fourer1987ampl}. 
It now also offers a complete tool set including many solvers for modeling different optimization problems.

Our optimization problem used to involve much more than just deducing log-likelihood functions before utilizing APML. 
Special effort had to be expanded to derive some components because of specific requirements from solving algorithms. 
For example, to apply IPOPT solver to our model estimation, we were required to sketch out all parameter derivatives of log-likelihood functions and Jacobian matrix. 
AMPL, however, allows us to solve the problem by only defining the problem and formulating the constraints.

To run AMPL on models, it needs two parts as input including model files and data files. Model files define the problem, while data files specify constants and initial values for variables. AMPL translator will read in those files and translate them into languages that solvers can understand. 
AMPL is particularly notable for its general syntax, including variable definitions and data structures. 
%\textcolor{red}{give a code snippet as example?} -- MAR: not necessary

\subsection{Used solvers and optimization setup}
\label{subsec:optimization-setup}
AMPL supports a comprehensive set of solvers including solvers for linear programming, quadratic programming and non-linear programming~\cite{fourer1993ampl}. 
This link\footnote{\url{http://www.ampl.com/solvers.html}} gives a full list of solvers for AMPL. 

\textbf{Solvers Applied in Implementation}.
%In the implementation for solving our model, we applied two solvers:
We used two solvers in our fitting procedure:
\begin{itemize}
%	\item \textbf{MINOS}: a large-scale optimization system designed for linear and non-linear problems \cite{murtagh1983minos}. The objective function may be linear or non-linear. However, the non-linear function must be smooth. Otherwise, it may stuck in local optimization and produce less reliable results. This is a default solver shipped with AMPL.
    \item \textbf{LGO}: a \emph{global optimizer} for non-linear problems, which is capable of finding approximate solutions when the problems have multiple local optimal solutions (\cite{pinter1997lgo}). This is also one of the default solvers provided by AMPL.
    \item \textbf{IPOPT}: an open-source large-scale \emph{local optimizer} for non-linear programming, which is released in 2006~\cite{Wachter2006}. 
\end{itemize}
Local solvers rely on improving an existing solution, employing complex techniques to avoid getting stuck in local minima.
They require an initial point from which to start exploring the space of solutions.
Global solvers attempt to search for the optimal solution in the entire space of solutions (one solution would be, for example, to divide the solution space into hyper-squares and apply local optimization in each one of them).
Global solvers tend to find solutions which are not too far from the optimal, but they lack the precision of specialized local solvers
In summary: local solvers achieve solutions very close to the optimal, but run the risk of getting stuck in horrible local optima;
global solvers achieve imprecise solutions close to the optimal.

%\verify{Not actually true! We don't user MINOS, we use only IPOPT as a local optimizer and LGO as a global optimizer.
%We have:
%\begin{itemize}
%	\item 8 random initializations within the definition range of parameters + IPOPT;
%	\item LGO + IPOPT to take advantage of LGO global search + IPOPT's local optimization;
%	\item IPOPT without starting parameters -- IPOPT has an internal strategy of choosing the starting point for the optimization, based on the parameters' range of definition.
%\end{itemize} }

\textbf{Optimization implementation setup}. 
Our optimization setup is constructed to account for the weaknesses of each class of solvers.
A classical solution to the problem of local optima with local solvers is to repeat the function optimization multiple times, from different starting points.
We generate 8 random sets of initial parameters, within the definition range of parameters, and we use the IPOPT solver using each of these as initial point.
We also combine the global and the local solver: we use LGO to search in the space of solutions for an approximate solution, which we feed into IPOPT as initial point for further optimization.
Lastly, we run IPOPT without any initial parameters, leveraging IPOPT's internal strategy for choosing the starting point based on the parameters' range of definition.
After completing these 10 rounds of optimization, we select the solution with the maximum training log likelihood values.
This tends to be the combination of global and local optimizer (LGO + IPOPT).
%
%Because we have utilized three solvers with different capabilities, our implementation needs to decide a way to apply them and choose the best results. The log-likelihood functions are non-linear problems, so we defined our process in following steps:
%\begin{enumerate}
%	\item Maximizing the log-likelihood functions with IPOPT and we then have a set of fitted parameters $\Theta_{IPOPT}$ and a holdout log-likelihood function value $l_{IPOPT}$.
%    \item Optimizing the log-likelihood functions with LGO which gives a fitted parameter set $\Theta_{LGO}$ and a holdout log-likelihood function value $l_{LGO}$.
%    \item Assigning $\Theta_{LGO}$ to corresponding log-likelihood functions as initial values, after which optimizing the functions with MINOS. This gives a fitted parameter set $\Theta_{LGO+MINOS}$ and a holdout log-likelihood function value $l_{LGO+MINOS}$.
%    \item Choose the parameters with the best holdout log-likelihood value among $l_{IPOPT}$, $l_{LGO}$ and $l_{LGO+MINOS}$.
%\end{enumerate}
%The reason we paired LGO and MINOS is that LGO is global optimizer whose result might be further improved by MINOS as a local optimizer.

\subsection{Interfacing AMPL with R}
\label{subsec:ampl-r-interface}
Our entire code base is using the R language, but AMPL has its own modeling language. 
Therefore, we need to interface between R and AMPL. 
Inspired by a blog post\footnote{\url{https://www.rmetrics.org/Rmetrics2AMPL}}, we implemented our own interface between AMPL and R language. The core ideas are described as follow:
\begin{itemize}
	\item \textbf{Generating model files and data files}: one of the major components of this interface is to generate temporary model and data files, which express the problem to be solved and the used data into AMPL language. 
	As our experiments involve a large amount of cascades, we prefixed all temporal files with process ids so that running AMPL in parallel becomes possible.
    \item \textbf{Interacting with AMPL}: this is also implemented by file I/O in the disk. After model files and data files are generated, we call AMPL via system commands through R and AMPL will then start optimization. Selections of solvers can be specified in the system commands used for starting AMPL. Optimization results will be saved in result files and our interface will extract results and return them.
    \item \textbf{Exception handling}: this is another important component of this interface as solvers are easily encountering errors during optimization process (such as computing $log(0)$) when float number running out of precision. 
\end{itemize}

\section{Relation between deterministic SIR and stochastic SIR}

\citet{Allen2008} analyzes in details the relation between the deterministic SIR and the stochastic SIR and shows that the mean behavior of the stochastic version converges asymptotically to the deterministic version.
She shows that the mean of the random function $I(t)$ in the stochastic SIR epidemic process is less than the solution $I(t)$ to the deterministic differential equation in~Eq.\eqref{eq:det-sir-size}.
We study the equivalence of the two flavors of SIR through simulation.
We simulate 100 realizations of the stochastic SIR and the deterministic SIR from the same set of parameters.
Fig.~\ref{fig:stochastic-vs-deterministic-SIR} shows the sizes of the population of Susceptible $S(t)$, Infected $I(t)$, Recovered $R(t)$ and the cumulated infected $C_t$.
For the stochastic version, we show the median and the 2.5\% / 97.5\% percentiles.
This result complements the analysis in Sec.~\ref{subsec:sir-model}.

%!TEX root = sir-hawkes.tex

\begin{figure}[tbp]
	\centering
	\newcommand\myheight{0.18}
	\subfloat[] {
		\includegraphics[page=1,height=\myheight\textheight]{stochastic-vs-deterministic-sir}
%		\label{subfig:popularity-scale-90}
	}
	\subfloat[] {
		\includegraphics[page=2,height=\myheight\textheight]{stochastic-vs-deterministic-sir}
%		\label{subfig:popularity-scale-120}
	}  \\
	\subfloat[] {
		\includegraphics[page=3,height=\myheight\textheight]{stochastic-vs-deterministic-sir}
%		\label{subfig:popularity-scale-jump}
	}
	\subfloat[] {
		\includegraphics[page=4,height=\myheight\textheight]{stochastic-vs-deterministic-sir}
%		\label{subfig:popularity-scale-jump}
	}
	\caption{ 
		We simulate 100 stochastic SIR realizations using the parameters $N = 1300, I(0) = 300, \beta = 1, \gamma = 0.2$.
		We show the median and the $2.5\%$ and $97.5\%$ percentile and the deterministic evolution simulated with the same parameters.
		We also show an example of stochastic realization.
	}
	\label{fig:stochastic-vs-deterministic-SIR}
\end{figure}
\input{5-simulation-fitting}

\section{Robustness of fit -- additional graphics}
Fig.~\ref{fig:robustness-fit-extra-graphs} shows the robustness of fit for parameters $\kappa$, $\beta$ and $\theta$ for Hawkes \emph{(a)-(c)} and HawkesN \emph{(d)-(f)}.
This result complements Sec.~\ref{subsec:robustness-of-fit}.

\begin{figure}[tbp]
	\centering
	\newcommand\myheight{0.2}
	\subfloat[] {
		\includegraphics[page=1,height=\myheight\textheight]{robustness-HAWKES}
	}
	\subfloat[] {
		\includegraphics[page=2,height=\myheight\textheight]{robustness-HAWKES}
	}\\
	\subfloat[] {
		\includegraphics[page=3,height=\myheight\textheight]{robustness-HAWKES}
	}
	\subfloat[] {
	\includegraphics[page=1,height=\myheight\textheight]{robustness-HAWKESN}
	}\\
	\subfloat[] {
		\includegraphics[page=2,height=\myheight\textheight]{robustness-HAWKESN}
	}
	\subfloat[] {
		\includegraphics[page=3,height=\myheight\textheight]{robustness-HAWKESN}
	}
	\caption{ 
		 Robustness of estimating parameters $\kappa$, $\beta$ and $\theta$ for Hawkes \emph{(a)-(c)} and HawkesN \emph{(d)-(f)}.
		One set of parameters for each model was simulated 100 times and fitted on increasingly longer prefixes of each simulation.
		One value for parameter is obtained for each fit and the median and the 15\%/85\% percentile values are shown.
	}
	\label{fig:robustness-fit-extra-graphs}
	\captionmoveup
\end{figure}

\section{Generalization performance -- Hawkes}
Fig.~\ref{fig:news1k-increasing-perc} shows the generalization performance of Hawkes, for increasing amounts of data.
Each cascade in a random sample of 1000 cascades in \News is observed for increasing periods of time.
This result complements the analysis in Sec.~\ref{subsec:explain-holdout}.

\begin{figure}[tbp]
	\centering
	\newcommand\myheight{0.18}
	\includegraphics[page=1,width=0.45\textwidth]{News1k-holdout-ll-increasing-perc}
	\caption{ 
		Performances of Hawkes explaining unobserved data, using holdout negative log likelihood.
		The performance over 1000 randomly sampled cascades in \News are summarized using boxplots, lower is better.
        The percentage of observed events in each cascade used to train Hawkes is varied between 10\% and 95\%.
	}
	\label{fig:news1k-increasing-perc}
	\captionmoveup
\end{figure}
